# Supplementary material for: Glueballs in Flatland
Source: arXiv:0710.2309 source file (2007-10-11)
Supplement: Supplementary file 1 [file appendix.tex]

\chapter{Appendix}

Etc.
